# Supplementary material for: Accelerating Neural Architecture Search via Proxy Data
Source: arXiv:2106.04784 source file (2021-06-09)
Supplement: Supplementary file 1 [file 8_appendix_imagenet.tex]

\begin{table*}[h]
    \begin{threeparttable}
    \centering
    \caption{Comparison with state-of-the-art neural networks on ImageNet (under mobile setting).}
    
        \begin{tabular}{lccccc}
            \toprule
            \multirow{2}{*}{\textbf{Neural Network}} & \multicolumn{2}{c}{\textbf{Test Err. (\%)}} & \textbf{Params.} & \textbf{Search Cost} & \textbf{Search Method} \\
            \cline{2-3}
             & \textbf{top-1} & \textbf{top-5} & \textbf{(M)} & \textbf{(GPU days)} \\
            \hline
            % hand-crafted
            % resnet?
            MobileNet~\cite{howard2017mobilenets} & 29.4 & 10.5 & 4.2 & - & manual \\
            ShuffleNet 2$\times$ (g=3)~\cite{zhang2018shufflenet} & 26.4 & 10.2 & $\sim$ 5 & - & manual \\
            \hline
            % NAS
            NASNet-A~\cite{zoph2018nasnet} & 26.0 & 8.4 & 5.3 & 1800 & RL \\
            AmoebaNet-A~\cite{real2019regularized} & 25.5 & 7.6 & 5.1 & 3150 & EA \\
            PNAS~\cite{liu2018progressive} & 25.8 & 8.1 & 5.1 & 225 & SMBO$^\ddag$ \\
            EcoNAS~\cite{zhou2020econas} & 25.2 & - & 4.3 & 8 & EA \\
            \hline
            % differentiable NAS
            DARTS (2nd order)~\cite{yang2019darts} & 26.7 & 8.7 & 4.7 & 1.06 & gradient \\
            SNAS (mild)~\cite{liang2019snas} & 27.3 & 9.2 & 4.3 & 1.5 & gradient/one-shot \\
            GDAS~\cite{dong2019searching} & 26.0 & 8.5 & 5.3 & 0.21 & gradient/one-shot \\
            ProxylessNAS (GPU)$^\ast$~\cite{han2019proxylessnas} & 24.9 & 7.5 & 7.1 & 8.3$^\dagger$ & RL or grad./one-shot \\
            PC-DARTS$^\ast$~\cite{xu2020pcdarts} & 24.2 & 7.3 & 5.3 & 3.8$^\dagger$ & gradient \\
            TuNAS$^\ast$~\cite{bender2020tunas} & 25.0 & - &  - & - & gradient/one-shot \\
            SDARTS-ADV~\cite{chen2020stabilizing-darts} & 25.2 & 7.8 & 4.8 &  1.3 & gradient \\
            FairDARTS-A~\cite{chu2019fairdarts} & 26.3 & 8.3 & 3.6 & 0.4 & gradient\\
            \hline
            % proposed (proxy dataset)
            \pddarts~($D_\mathrm{rnd}$, 128k) & 25.6 & 8.1 & 4.4 & \textbf{0.56}$^\dagger$ & gradient \\
            \pddarts~(20k+108k) & 24.8 & 7.7 & 5.1 & \textbf{0.56}$^\dagger$ & gradient \\
            \pddarts~(25k+103k) & 25.1 & 7.8 & 4.9 & \textbf{0.56}$^\dagger$ & gradient \\
            \bottomrule
        \end{tabular}
        \begin{tablenotes}
            \small
            \item $^\dagger$This neural network was directly searched on ImageNet, otherwise searched on CIFAR-10 or CIFAR-100 and then transferred. Notably, \pddarts~can search using single V100 GPU for approximately 13 GPU hours.
            \item $^\ast$ProxylessNAS and TuNAS used 100\% of training examples of ImageNet; PC-DARTS used 10\% and 2.5\% of training examples of ImageNet for $D_{\mathrm{tr}}$ and $D_{\mathrm{val}}$ in Eq.~\ref{eq:NAS_formula}.
            \item $^\ddag$ is an abbreviation of the sequential model-based optimization.
        \end{tablenotes}
        \vspace{-0.7em}
    \label{table:imagenet_full_comparison}
    \end{threeparttable}
\end{table*}
